# Supplementary material for: Robustness of Safety for Linear Dynamical Systems: Symbolic and Numerical Approaches
Source: arXiv:2109.07632 source file (2021-09-16)
Supplement: Supplementary file 1 [file appendix.tex]

\section{Ordering Cells based on sensitivity to perturbation}
\label{apx:orderEval}

\subsection{Flight Envelope} In \cite{inproceedings}, the effect of cells on the perturbation at time step 100 with initial set $[-1,1] \times [-1,1] \times [-1,1] \times [-1,1] \times [-1,1] \times [-1,1] \times [-1,1] \times [-1,1] \times [-1,1] \times [-1,1] \times [-1,1] \times [-1,1] \times [1,1] \times [1,1] \times [1,1] \times [1,1]$ is shown in figure \ref{fig:flightOrd}. In this is example, there is no visible effect of perturbation in bottom 5 cells. 

\begin{figure}
\centering
\includegraphics[width=7cm,height=5cm]{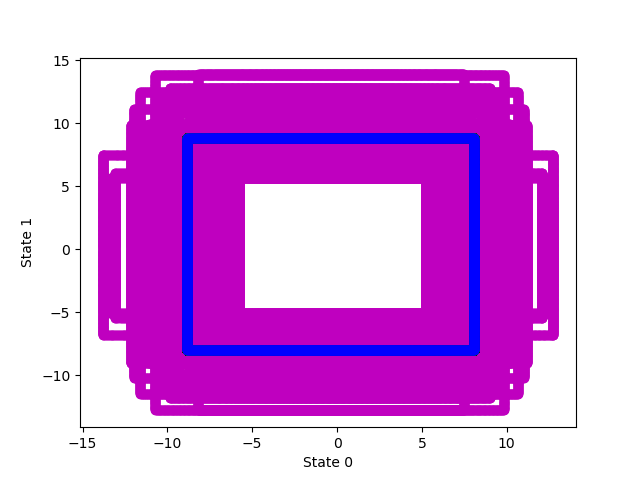}
\caption{Effect of cells on reachable set at time step 100.}\label{fig:flightOrd}
\end{figure}

\section{Evaluation on Benchmarks}
\label{apx:eval}

\subsection{A PK/PD Model}
\label{subsec:pkpd}
In \cite{ARCH15:Benchmark_Problem_PK_PD_Model}, a 5 dimensional system, we introduce perturbation of $\pm 20$ \% in weight of the child and $k_d$. We chose our initial set as [1,6] $\times$ [0,10] $\times$ [0,10] $\times$ [1,8] $\times$ [0,200]. The reachable sets at time step 1950 returned by our numerical approach is visualized (States $\tilde{c}_1$, $\tilde{c}_2$) in fig. ~\ref{fig:PKPD} (Right). The computation time taken by our numerical method up to 2050 steps is given in table \ref{tab:results1}. Using our symbolic approaches, we computed the bloating factors from time 50 to 55 with step size of 0.01. For this benchmark, we observed that the bloating factor returned by \texttt{Kagstrom2} explodes, so we excluded that from the result. The result of the bloating factor computation are shown in fig. \ref{fig:PKPD} (Left), and the timing details can be found in table \ref{tab:results2}. The ordering of the top 5 cells as returned by our approach, with decreasing sensitivity to perturbation are \{(1, 1), (2, 2), (3, 3), (4, 4), (0, 0)\}. The time taken to compute the ordering of all the cells are given in table \ref{tab:results3}.

\begin{figure}
\centering
\includegraphics[width=12cm,height=4.2cm]{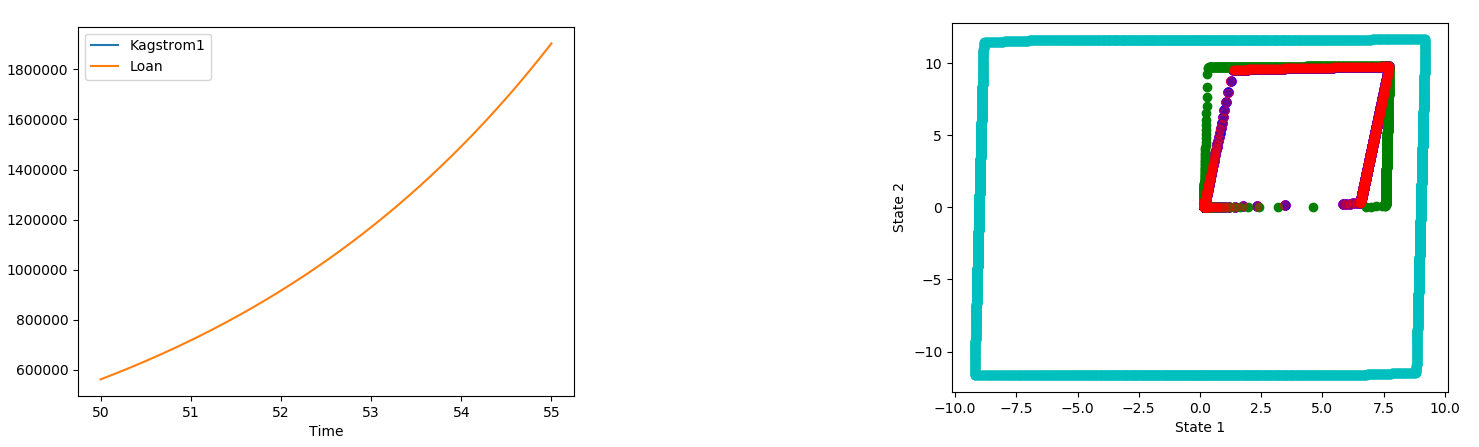}
\caption{(Left) Bloating Factors of PK/PD, (Right) Reachable sets of PK/PD at time step 1950}\label{fig:PKPD}
\end{figure}

%\begin{figure}
%\centering
%\includegraphics[width=7cm,height=5cm]{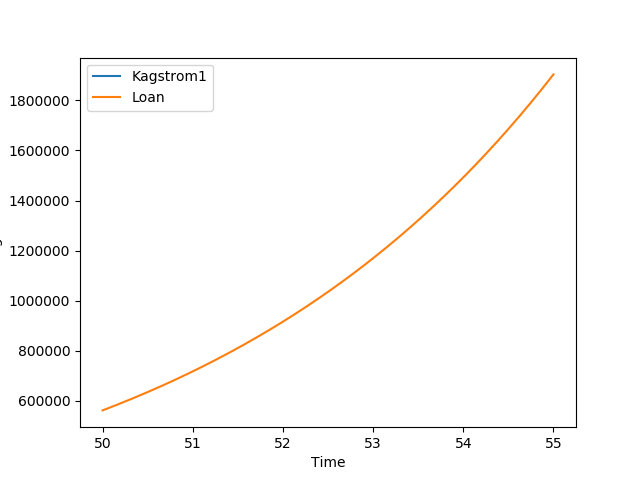}
%\caption{Bloating Factors of PK/PD}\label{fig:PKPDBloat}
%\end{figure}

\subsection{Motor-Transmission Drive System}
\label{subsec:motor1}
In \cite{ARCH15:Motor_Transmission_Drive_System_Benchmark}, a 7 dimensional system, we introduce perturbation of $\pm 20$ \% in in cells \{(0,6), (1,6)\}. We chose our initial set as [-1,1] $\times$ [-1,1] $\times$ [-1,1] $\times$ [-1,1] $\times$ [-1,1] $\times$ [1,1] $\times$ [1,1]. The reachable sets at time step 1950 returned by our numerical approach is visualized (States $v_x$, $v_y$) in fig.~\ref{fig:Motor1} (Right). The computation time taken by our numerical method up to 2050 steps is given in table \ref{tab:results1}. Using our symbolic approaches, we computed the bloating factors from time 50 to 100 with step size of 0.01. The result of the bloating factor computation are shown in fig. \ref{fig:Motor1} (Left), and the timing details can be found in table \ref{tab:results2}. The ordering of the top 5 cells as returned by our approach, with decreasing sensitivity to perturbation are \{(4, 4), (3, 3), (2, 2), (0, 0), (1, 1)\}. The time taken to compute the ordering of all the cells are given in table \ref{tab:results3}.

\begin{figure}
\centering
\includegraphics[width=12cm,height=4.2cm]{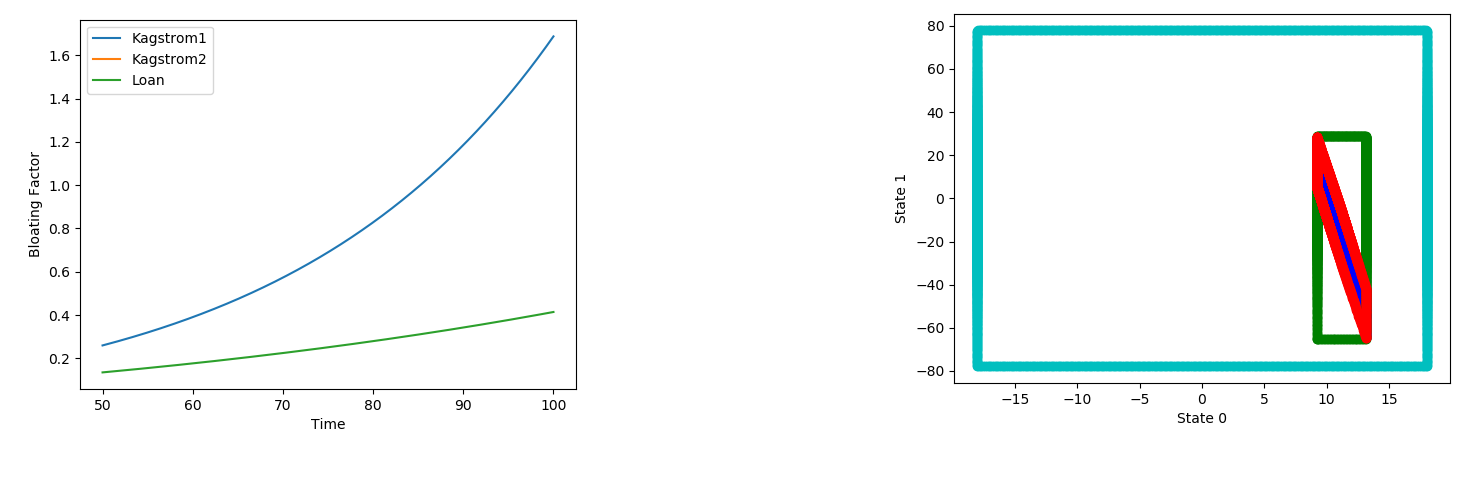}
\caption{(Left) Bloating Factors of Motor Transmission, (Right) Reachable sets of Motor Transmission at time step 1950.}\label{fig:Motor1}
\end{figure}

%\begin{figure}
%\centering
%\includegraphics[width=7cm,height=5cm]{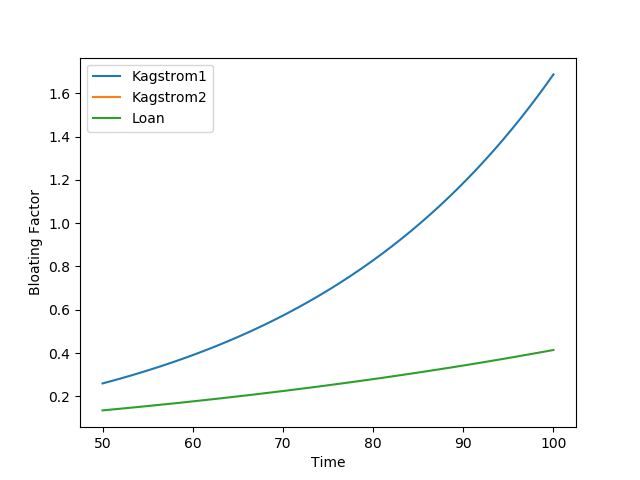}
%\caption{Bloating Factors of Motor Transmission}\label{fig:Motor1Bloat}
%\end{figure}

\subsection{Girad I}
\label{subsec:girdaI}
In
\cite{10.1007/978-3-540-31954-2_19},
a 2 dimensional system, we introduce perturbation of $\pm 2$ \% in in cells \{(0,0), (1,0)\}. We chose our initial set as $[0.9,1.1] \times [-0.1,0.1]$. The reachable sets returned by our numerical approach is visualized in fig.~\ref{fig:GiradI} (Right). The computation time taken by our numerical method up to 2050 steps is given in table \ref{tab:results1}. Using our symbolic approaches, we computed the bloating factors from time 0 to 2 with step size of 0.01. The result of the bloating factor computation are shown in fig. \ref{fig:GiradI} (Left), and the timing details can be found in table \ref{tab:results2}. The time taken to compute the ordering of all the cells are given in table \ref{tab:results3}.

\begin{figure}
\centering
\includegraphics[width=12cm,height=4.2cm]{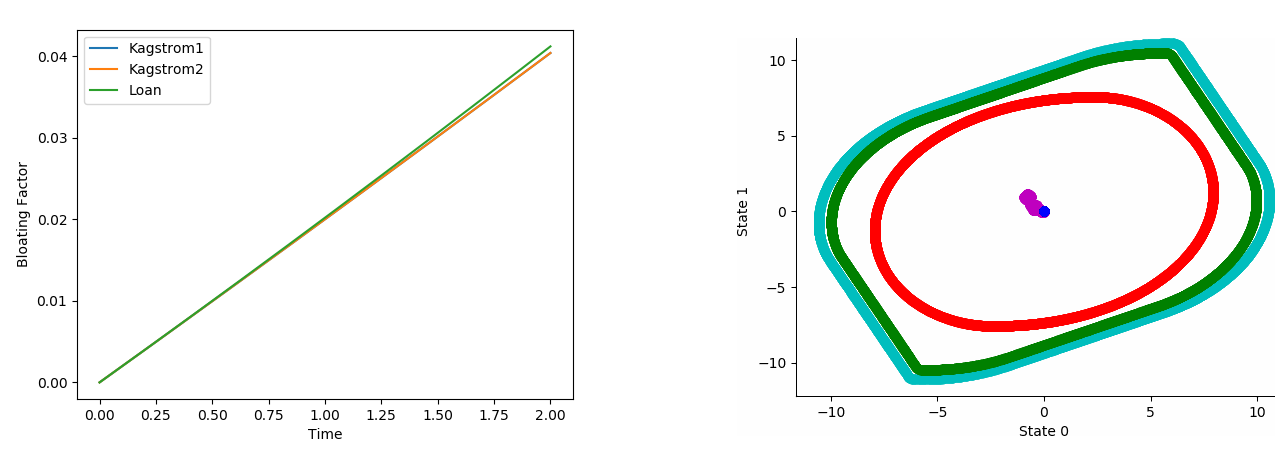}
\caption{(Left) Bloating Factors of Girad I, (Right) Reachable sets of Girad I.}\label{fig:GiradI}
\end{figure}

%\begin{figure}
%\centering
%\includegraphics[width=7cm,height=5cm]{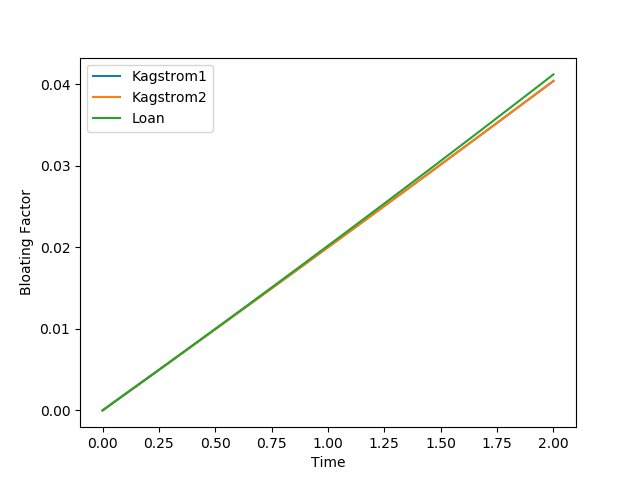}
%\caption{Bloating Factors of Girad I}\label{fig:GiradBloat}
%\end{figure}

\begin{table}
    \centering
    \resizebox{260pt}{!}{%
    \begin{tabular}{| c | c | c | c | c |}
    \hline
~Benchmark~ & ~Dim~ & \texttt{Kagstrom1}~ & ~\texttt{Kagstrom2}~ &  ~ \texttt{Loan}~\\ \hline
Holes & 10 & 0.004 s & 0.4 s & 0.004 s \\ \hline
ACC & 4 &  0.02 s & 0.06 s & 0.014 s \\
\hline
Lane Change & 7 & 0.007 s & 0.29 s & 0.001 s \\
\hline
PK/PD & 5 & 0.005 s & 9.06 s & 0.0012 s \\
\hline
Motor & 7 & 0.06 s &  0.11 s & 0.008 s \\
\hline
Girad I & 2 & 0.002 s & 0.02 s & 0.001 s \\
\hline
Girad II & 5 & 0.002 s & 0.28 s & 0.0006 s \\
\hline
Space & 6 & 0.002 s & 0.2 s & 0.0006 s \\
\hline
Aircraft & 4 & 0.01 s & 0.04 s & 0.01 s \\
\hline
CoOp I & 10 & 0.004 s & -  & 0.0008 s \\
\hline
Flight & 16 & 0.03 s & 2.009 s & 0.002 s \\
\hline
5-Veh & 15 & 0.002 s & -  & 0.0006 s \\
\hline

    \end{tabular}%
    }
     \caption{Time taken by the numerical approach for 2050 steps. \textbf{Dim}: Dimensions of the system, \textbf{\texttt{Kagstrom1}}: Time taken by Kagstrom1, \textbf{\texttt{Kagstrom2}}: Time taken by Kagstrom2, \textbf{\texttt{Loan}}: Time taken by Loan}
    \label{tab:results2}
\end{table}
\begin{table}
    \centering
    %\resizebox{380pt}{90pt}{
    \begin{tabular}{| c | c | c |}
    \hline
~Benchmark~ & ~Dim~ & ~Time~ \\ \hline
Holes & 10 & 0.01s \\ \hline
ACC & 4 & 0.0006 s \\
\hline
Lane Change & 7 & 0.004 s \\
\hline
PK/PD & 5 & 0.001 s \\
\hline
Motor & 7 & 0.004 s \\
\hline
Girad I & 2 & 0.0003 s \\
\hline
Girad II & 5 & 0.005 s \\
\hline
Space & 6 & 0.002 s \\
\hline
Aircraft & 4 & 0.0008 s \\
\hline
CoOp I & 10 & 0.01 s \\
\hline
Flight & 16 & 0.2 s \\
\hline
5-Veh & 15 & 0.4 s \\
\hline

    \end{tabular}%}
     \caption{Time taken by our approach to order the cells of the matrix based on sensitivity to perturbation \textbf{Dim}: Dimensions of the system, \textbf{Time}: Time taken by our approach to find the ordering of all the cells}
    \label{tab:results3}
\end{table}
